# Supplementary material for: Redshifted 21-cm bispectrum II: Impact of the spin temperature fluctuations and redshift space distortions on the signal from the Cosmic Dawn
Source: arXiv:2012.11616 source file (2021-01-22)
Supplement: Supplementary file 1 [file appendix.tex]

%%%%%%%%%%%%%%%%% APPENDICES %%%%%%%%%%%%%%%%%%%%%

\appendix

\section{}
\label{sec:app1}
\comment{
\begin{figure*}
%\begin{minipage}[b]{0.47\textwidth}
  \includegraphics[width=0.24\textwidth,angle=0]{figures/cos-theta_k2byk1_mu1mu2.eps}
  \includegraphics[width=0.24\textwidth,angle=0]{figures/cos-theta_k2byk1_mu2mu3.eps}
   \includegraphics[width=0.24\textwidth,angle=0]{figures/cos-theta_k2byk1_mu1mu3.eps}
   \includegraphics[width=0.24\textwidth,angle=0]{figures/cos-theta_k2byk1_mu1mu2mu3.eps}
  
  \caption{These panels show the value of coefficients $[\overline{\mu_1^2 \mu_2^2}]_0^0$, $[\overline{\mu_2^2 \mu_3^2}]_0^0$, $[\overline{\mu_3^2 \mu_1^2}]_0^0$ and $[\overline{\mu_1^2 \mu_2^2 \mu_3^2}]_0^0$ in the equation \eqref{eq:b_qlin_multipole} for $m= 0,\, \ell=0$. This figure is same as Figure A1 of \citet{majumdar20}.}
  \label{fig:monopole}
%\end{minipage}
\end{figure*}
}
